# Supplementary material for: Accidental Light Probes
Source: arXiv:2301.05211 source file (2023-06-10)
Supplement: Supplementary file 1 [file supp_indoor.tex]

\begin{figure*}[t]
\centering
\includegraphics[width=\linewidth]{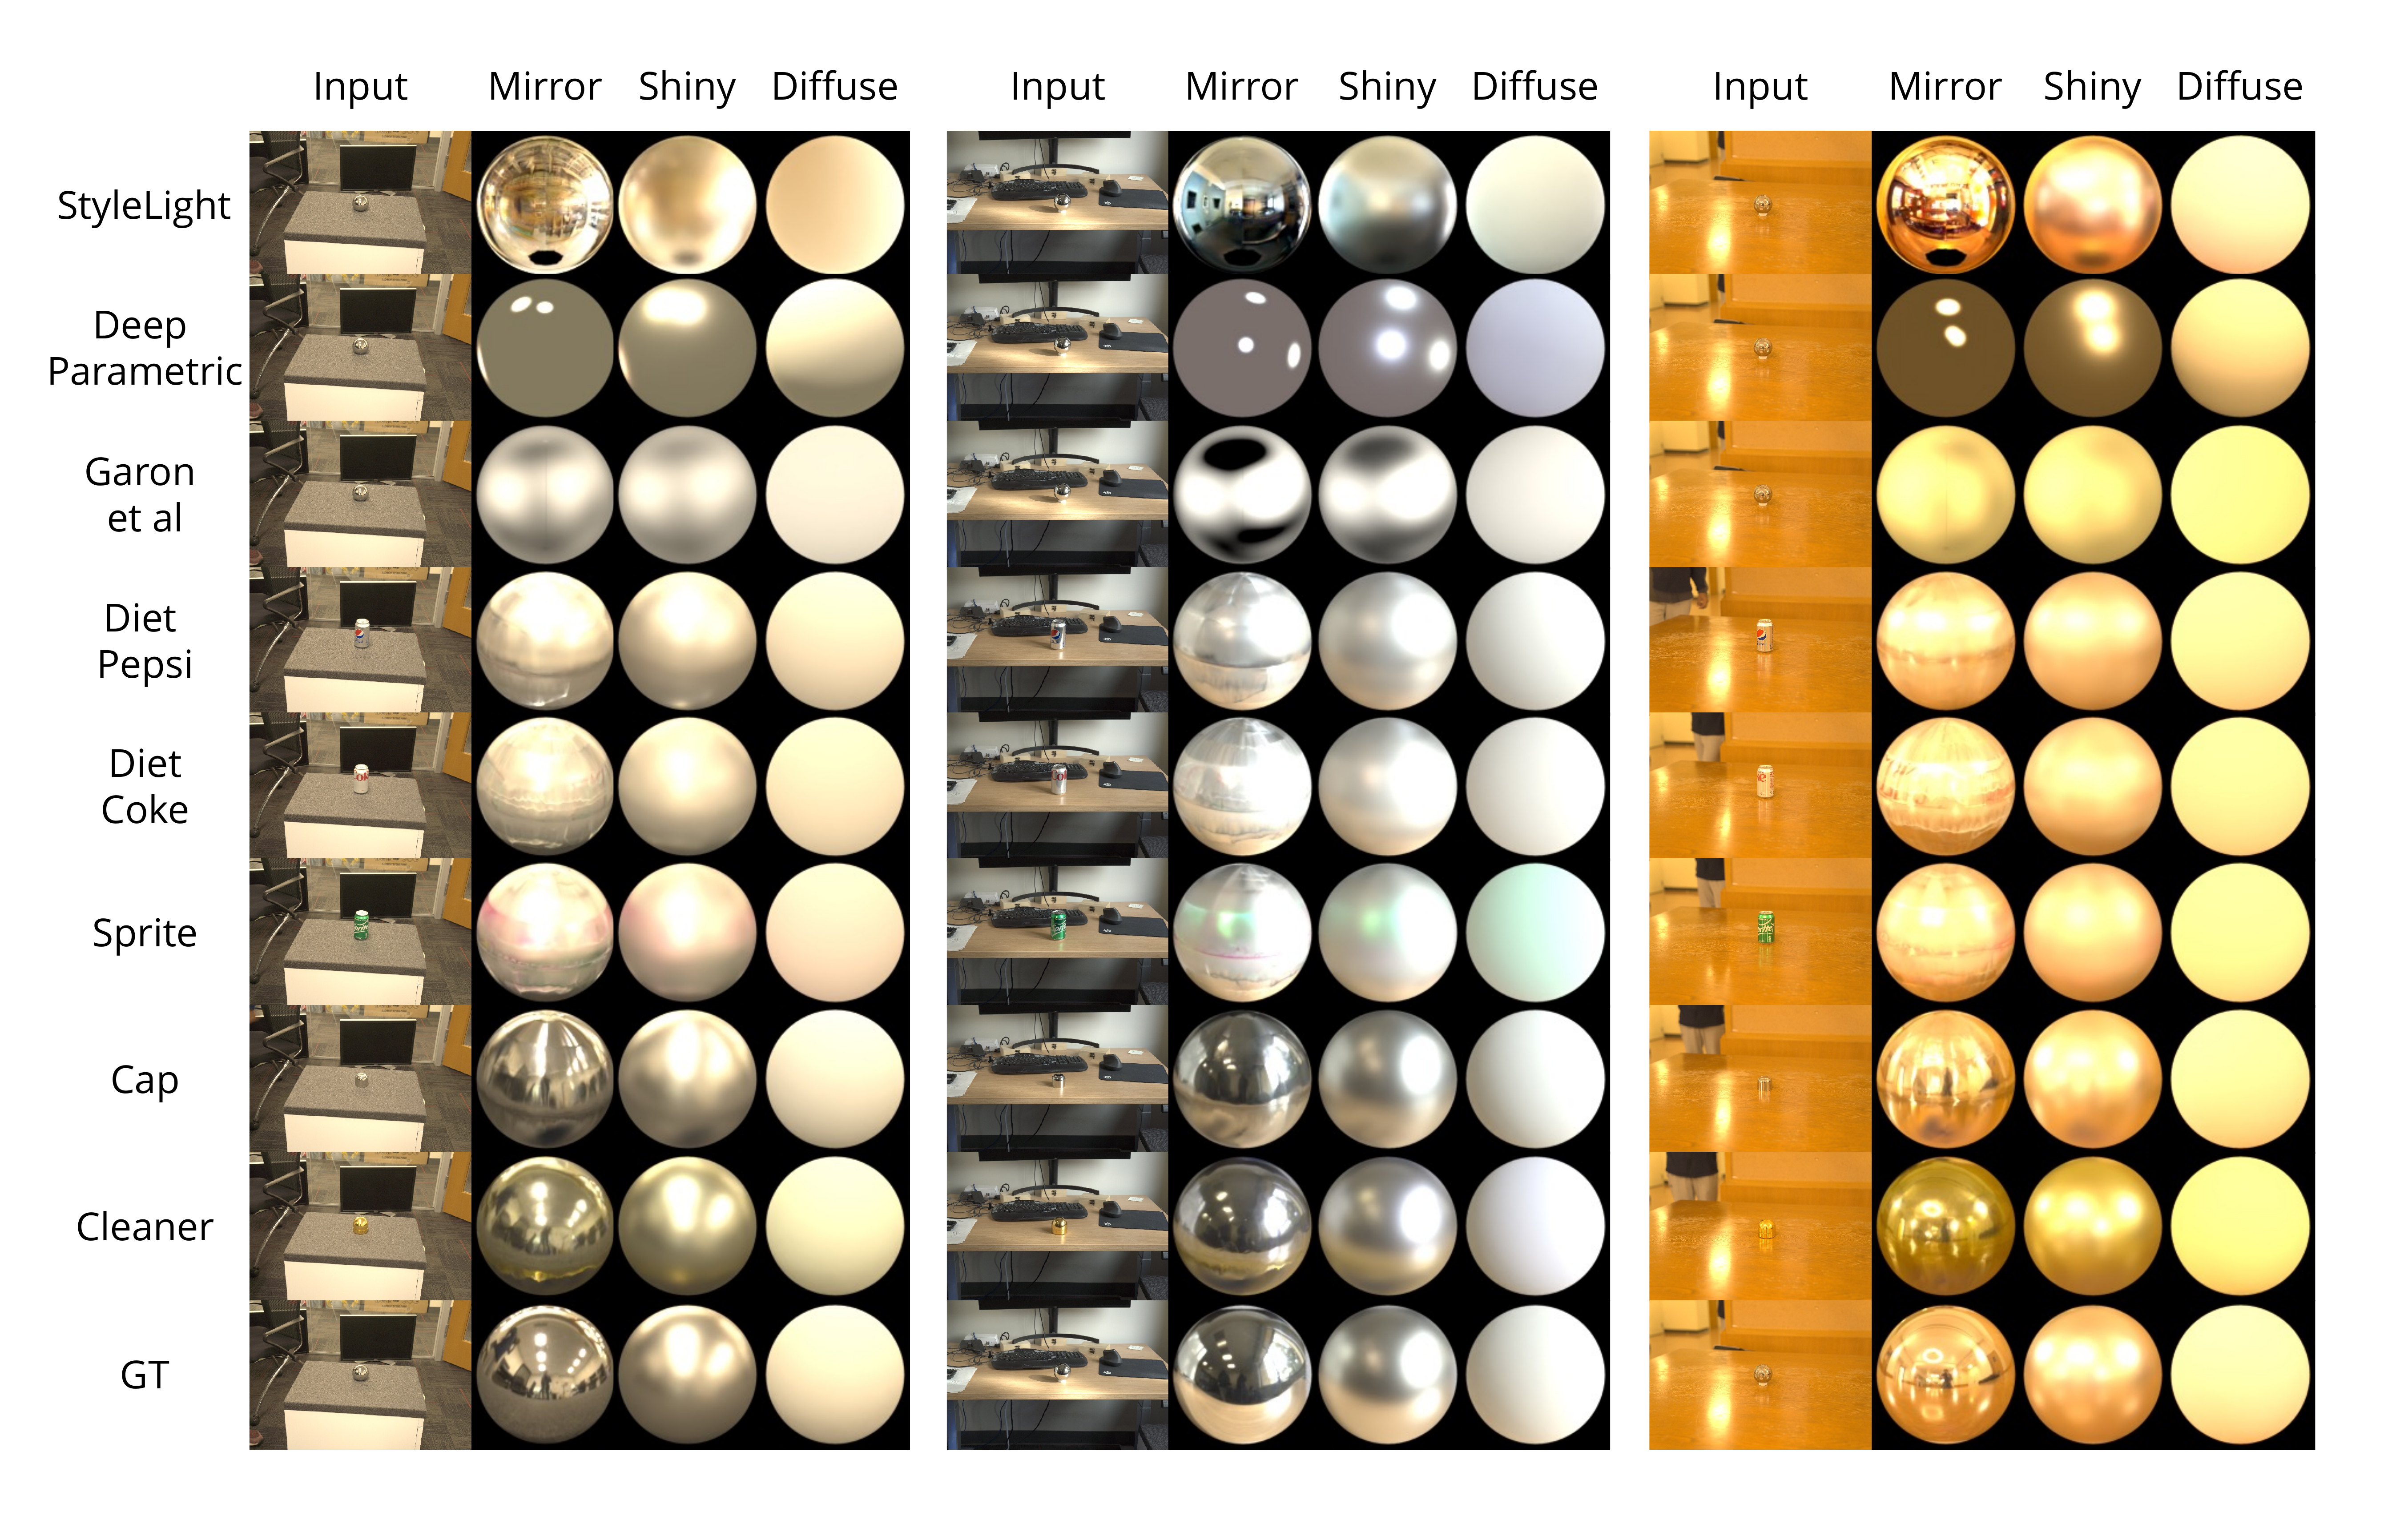}
\vspace{-0.2in}
\caption{Additional qualitative results for indoor scenes. We compare our approach to StyleLight~\cite{wang2022stylelight}, Deep Parametric~\cite{gardner2019deep} and Garon et al~\cite{garon2019fast} on relighting mirror, shiny and diffuse spheres.}
\label{fig:indoor_supp}
\end{figure*}
