# Supplementary material for: Accidental Light Probes
Source: arXiv:2301.05211 source file (2023-06-10)
Supplement: Supplementary file 2 [file supp_mat.tex]

\begin{figure*}[ht!]
\centering
\includegraphics[width=\linewidth]{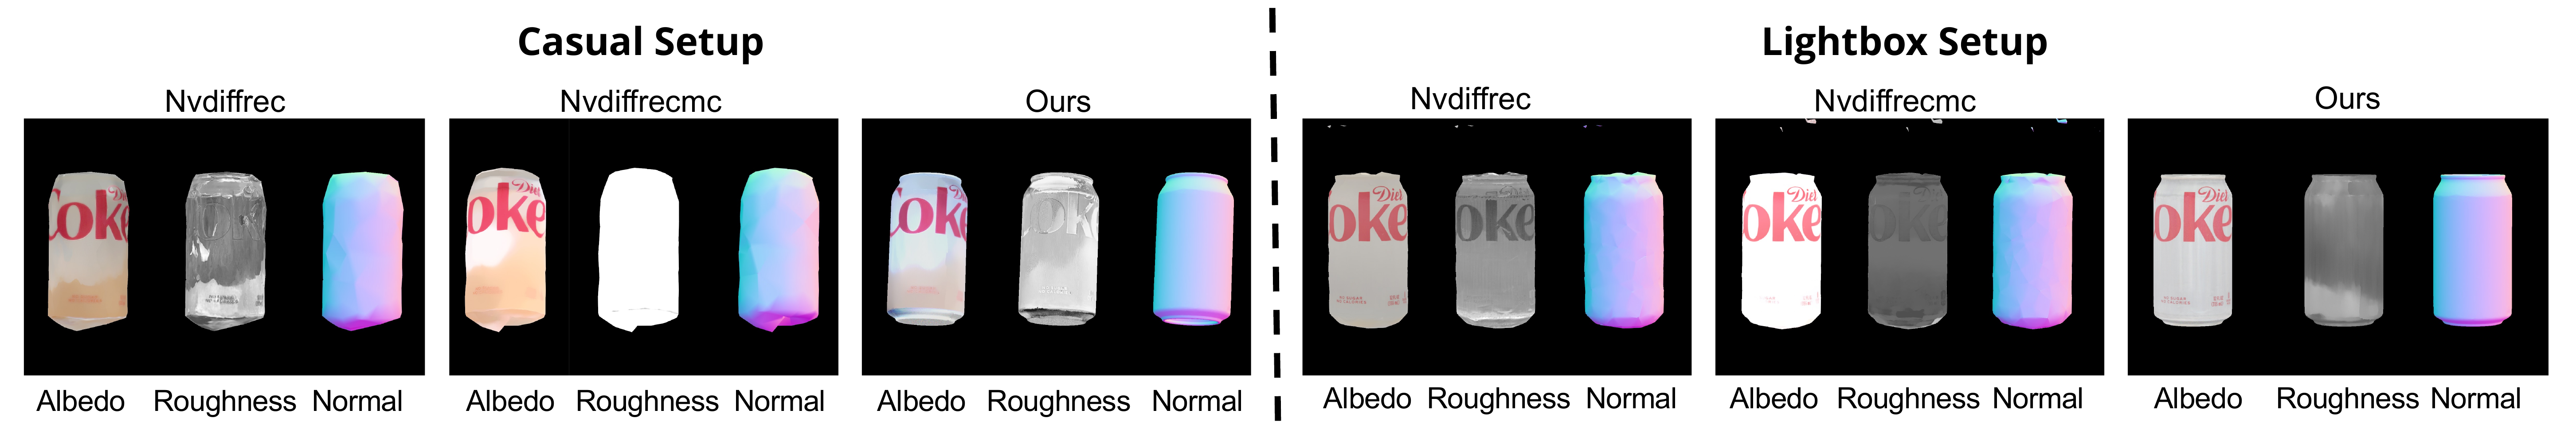}
\vspace{-0.3in}
\caption{Qualitative comparison of the materials and geometry of a Diet Coke can using our method and \cite{munkberg2022extracting, hasselgren2022shape} in both setups.}
\label{fig:mat_sup}
\end{figure*}
