# Supplementary material for: Accidental Light Probes
Source: arXiv:2301.05211 source file (2023-06-10)
Supplement: Supplementary file 4 [file supp_abl_casual.tex]

\begin{table*}[t]
    \centering
    \small
    \begin{tabular}{l|ccc|ccc}
        \toprule
        & \multicolumn{3}{c|}{Casual multi-view} & \multicolumn{3}{c}{Lightbox setup} \\
        Method  &  Mirror & Shiny & Diffuse  & Mirror & Shiny & Diffuse \\
        \midrule
        Nvdiffrec~\cite{munkberg2022extracting} & 12.23 & 10.99 & 9.14 & 6.99 & 5.06 & 3.59 \\
        Nvdiffrecmc~\cite{hasselgren2022shape} & 8.76 & 7.37 & \textbf{4.71} &  6.55 & 4.60 & 3.84 \\
        ALP (Ours) & \textbf{6.49} & \textbf{5.48} & 4.89  & \textbf{5.46} & \textbf{3.67} & \textbf{2.80} \\
        \bottomrule
    \end{tabular}
    \caption{Evaluation on our ALP model acquisition for a diet coke can under two different capture settings: casual multi-view images and our lightbox setup. We use the same lighting estimation approach for compared methods and report average angular error across all test scenes.}
    \label{tbl:supp_abl_casual}
\end{table*}
